# Supplementary material for: Guiding Neuroevolution with Structural Objectives
Source: arXiv:1902.04346 ancillary file (2019-04-23)
Supplement: Supplementary file 1 [file supplementary_material.pdf]

# Supplementary Material to: Guiding Neuroevolution with Structural Objectives

**Kai Olav Ellefsen** kaiolae@ifi.uio.no
Department of Informatics, University of Oslo, Norway

**Joost Huizinga** jhuizinga@uber.com
Uber AI Labs, USA

**Jim Torresen** jimtoer@ifi.uio.no
Department of Informatics, University of Oslo, Norway

---

| Parameter | Retina Problem | Robot Locomotion Problem |
|---|---|---|
| Number of generations | 5000 | 5000 |
| Population size | 1000 | 100 |
| Crossover | No | No |
| Mutations | Yes. See Supplementary Material Table 2. | Yes. See Supplementary Material Table 3 |

Table 1: Main parameters for the experiments. The population size in the robot locomotion problem is a compromise between solution quality and demand for computational resources. We found that with the current setting, final evolved individuals frequently reached high-quality locomotion patterns, as can be seen in the video linked to in the main text.

| Probability | Mutation Type |
|---|---|
| 20% (per network) | Adding a connection between two randomly chosen neurons. Neurons are required to be on consecutive layers and not already connected. |
| 20% (per network) | Removing a random connection. |
| $2/n$ | Changing the weight of one of the $n$ connections in the network, following the mutation from (Clune et al., 2013) for discrete-weight networks. |
| 15% (per connection) | Moving the source or target of a connection to another random neuron on the same layer. |
| $1/24 = 4.16\%$ (per node) | Changing the bias-input of the node, following the mutation from (Clune et al., 2013) for discrete-weight networks. |

Table 2: Mutational operators and probabilities for evolving neural networks in the Retina Problem, following the experimental setup in Clune et al. (2013).

| Probability | Mutation Type |
|---|---|
| 9% (per network) | Adding a connection between two randomly chosen nodes. |
| 8% (per network) | Removing a random connection. |
| 6% (per network) | Add a new node onto a randomly selected connection. The selected connection is replaced by one connection that goes from its source node to the new node and one connection that goes from the new node to its target node, both inheriting the weight of the selected connection. |
| 5% (per network) | Removing a random node. |
| 10% (per connection) | Changing the weight of a connection, applying polynomial mutation (Deb, 2001). After mutation, weights are clipped to lie between $-3$ and 3. |
| 10% (per node) | Mutate activation function, by drawing a new one from the available set of sine, identity, Gaussian, and sigmoid with uniform probability. |

Table 3: Mutational operators and probabilities for the evolving CPPNs in the robot locomotion problem, following the experimental setup in Huizinga et al. (2016).

This is the authors' final version. Article accepted for publication in MIT Press Evolutionary Computation Journal

| | |
|---|---|
| Neuron Potential ($\gamma$): | $\gamma_i^{t+1} = \gamma_i^t + \frac{1}{\tau_i}(-\gamma_i^t + \sum_{j=1}^{n} w_{ji} a_j^t)$ |
| Neuron Activation ($a$): | $a_i^t = tanh((b_i + \gamma_i^t)\lambda)$ |

Table 4: Equations for updating nodes in the CTRNN (Beer and Gallagher, 1992) from the spider robot experiment. $\gamma_i^t$ is the potential of neuron $i$ at time $t$, $\tau_i$ is the time constant of neuron $i$, $b_i$ is the bias of neuron $i$, $w_{ji}$ is the weight of the connection from neuron $j$ to neuron $i$, $a_i^t$ is the activation of neuron $i$ at time $t$, $n$ is the total number of neurons in the network, and $\lambda$ is a parameter that determines the steepness of the activation function ($\lambda = 5$ in this work).

| | |
|---|---|
| Hip up-down range: | $[-\frac{1}{4}\pi, \frac{1}{4}\pi]$ |
| Hip front-back range: | $[-\frac{1}{8}\pi, \frac{1}{8}\pi]$ |
| Knee range: | $[-\frac{1}{8}\pi, 0.2]$ |
| $desiredAngle$: | $a_i(r_i^{max} - r_i^{min}) + r_i^{min}$ |
| $velocity$: | $\frac{(desiredAngle - currentAngle)}{stepLength}$ |
| $stepLength$: | 0.01 |

Table 5: Parameters and equations for controlling the spider-robot actuators. Here, $a_i$ is the activation of output neuron $i$, $r_i^{min}$ and $r_i^{max}$ are the lower and upper bound of the actuator associated with output neuron $i$, respectively, and $stepLength$ is the amount of time simulated in a single simulator step.

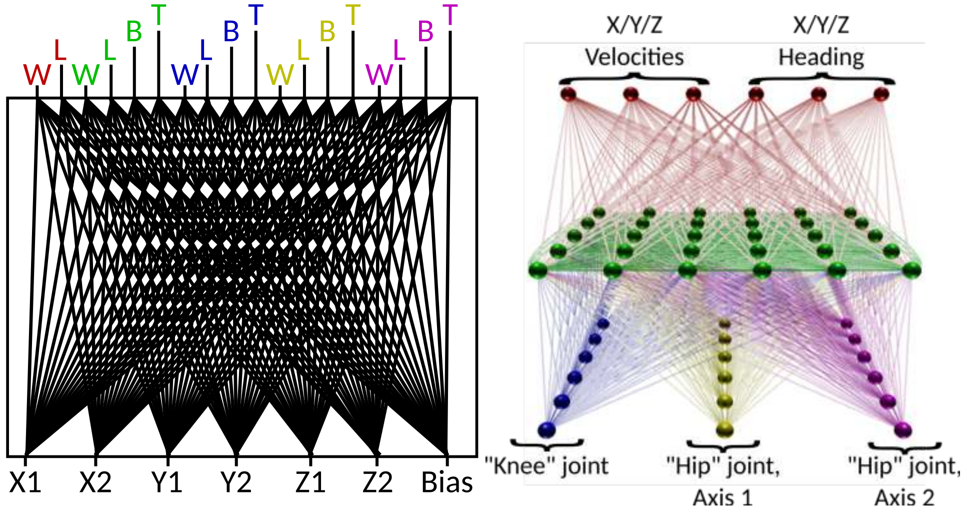


(a) Initial CPPN (b) Multi-spatial substrate

Figure 1: Left is the initial CPPN, which is fully connected with no hidden nodes. Inputs (bottom) are the coordinates of pairs of nodes in the substrate and a bias, and outputs (top) determine parameters of these nodes and their connections. The bias input is always 1 and it is added because the nodes in the CPPN do not have their own internal bias. Because the bias input is always one, the weight of the connection from the bias input to a CPPN node will act as the bias value for that node. The outputs are the weight output (W), the link expression output (L), the bias output (B), and the time-constant output (T). The different colors for the CPPN outputs indicate different *planes* as defined by the multi-spatial substrate (Pugh and Stanley, 2013). Each plane (colored set) of CPPN outputs defines the parameters of the nodes and connections with the same color in the network on the right, where the input layer, the hidden layer, and the three different actuator types in the output layer (knee, hip axis 1, and hip axis 2) are in separate planes (i.e. have different colors). These neurons are in separate planes because the spatial relationships between them are not obvious (e.g. the hidden layer has no obvious spatial relationship with respect to the inputs or outputs of the robot because the hidden layer is not a physical part of the robot), and dividing them into separate planes improved overall performance in preliminary experiments. The input set (red) does not have a bias an time-constant output because the input neurons do not have a bias or time constant. *Image adapted from Huizinga et al. (2016).*

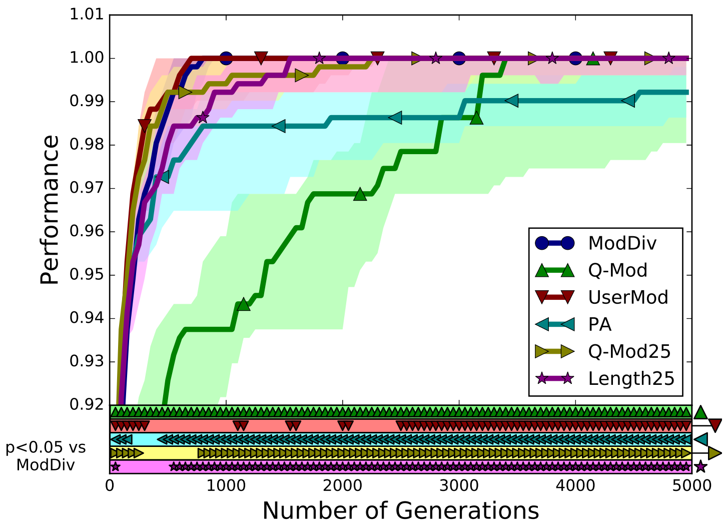


(a) Performance of the best individual

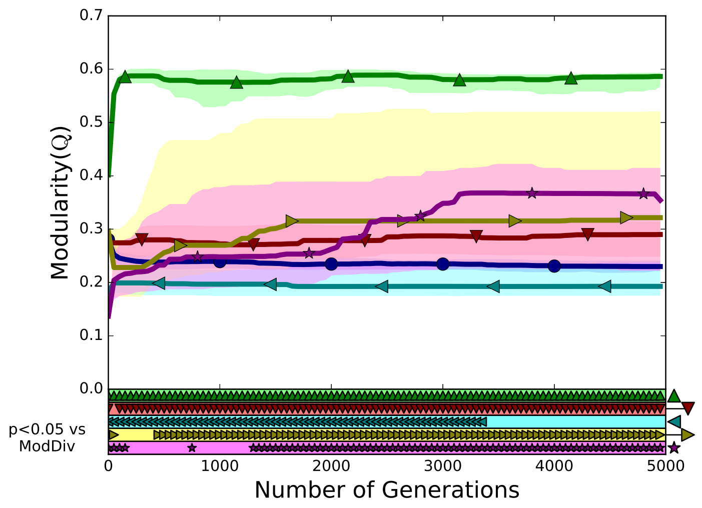


(b) Median population modularity (Q-score)

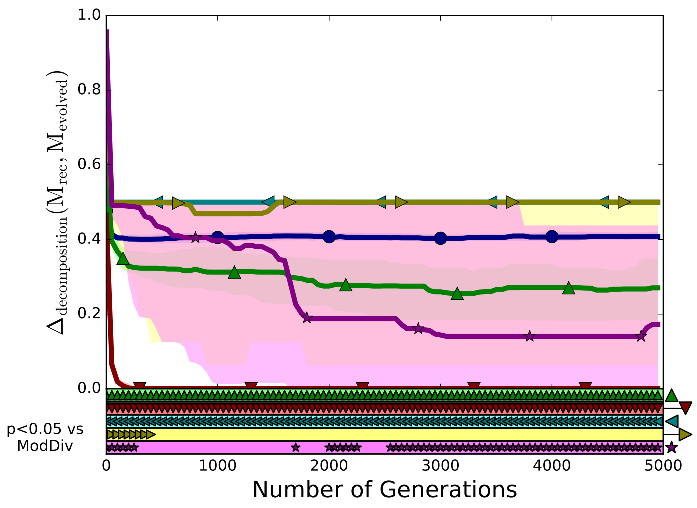


(c) Median population distance from $M_{rec}$

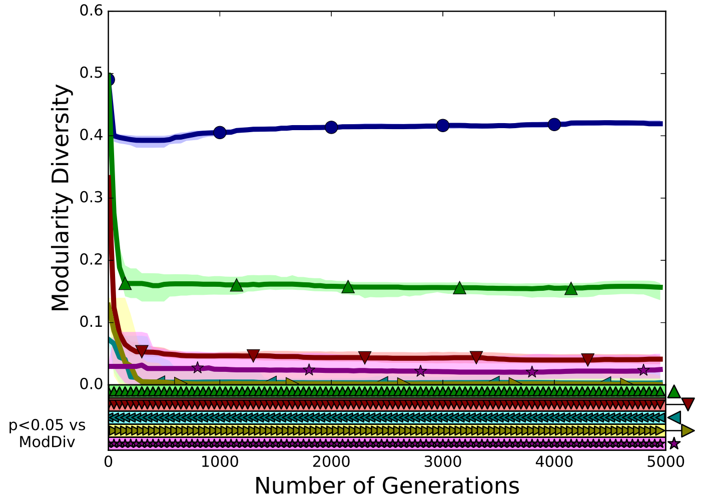


(d) Median population diversity.

Figure 2: The results from the Retina experiment, shown together with results replicating the setup from Clune et al. (2013), where a probabilistic version of NSGA-II was applied, which put less emphasis on structural objectives than the functional objective (*Q-Mod25* and *Length-25*). In agreement with Clune et al. (2013), we see this probabilistic version increase performance (versus *PA* and *Q-Mod*), but our new distance-based structural measures *ModDiv* and *UserMod* result in the best performance, despite these balancing structural and functional objectives evenly.

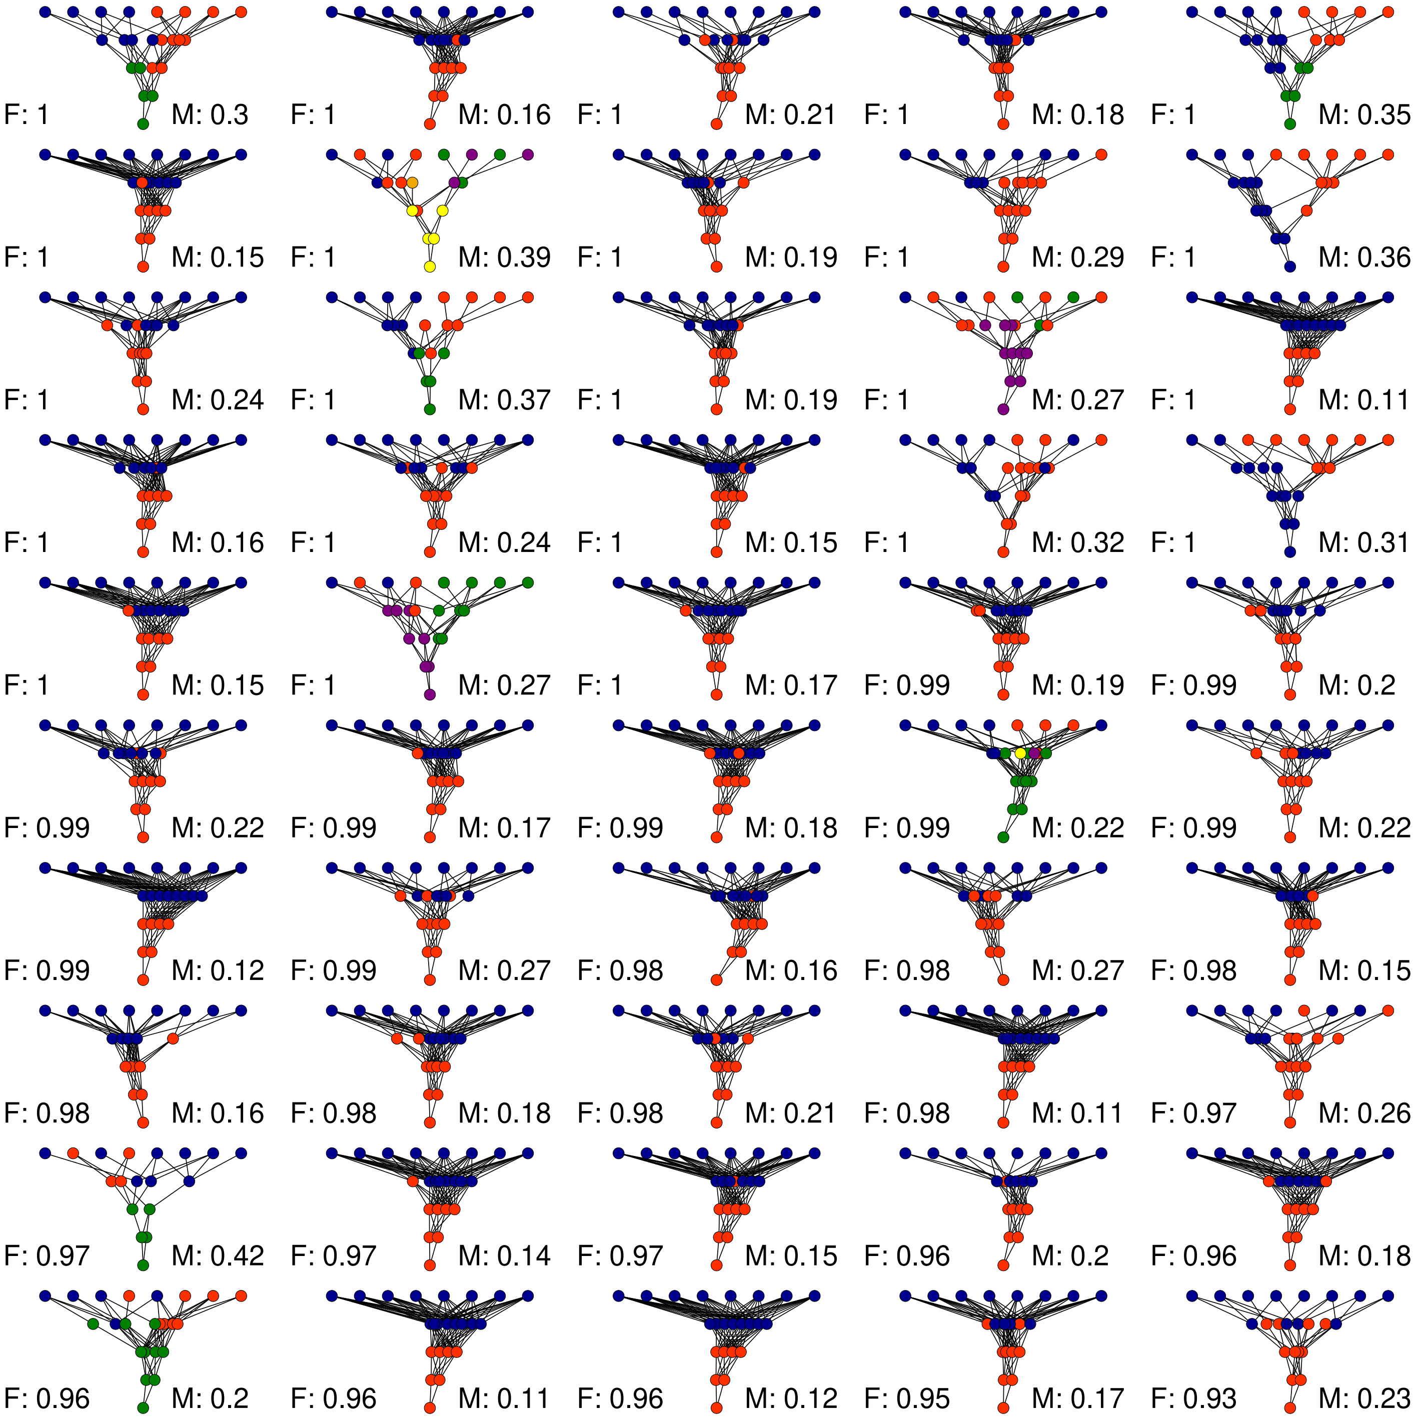


Figure 3: All 50 evolved neural networks from the retina experiment, with the *PA* treatment

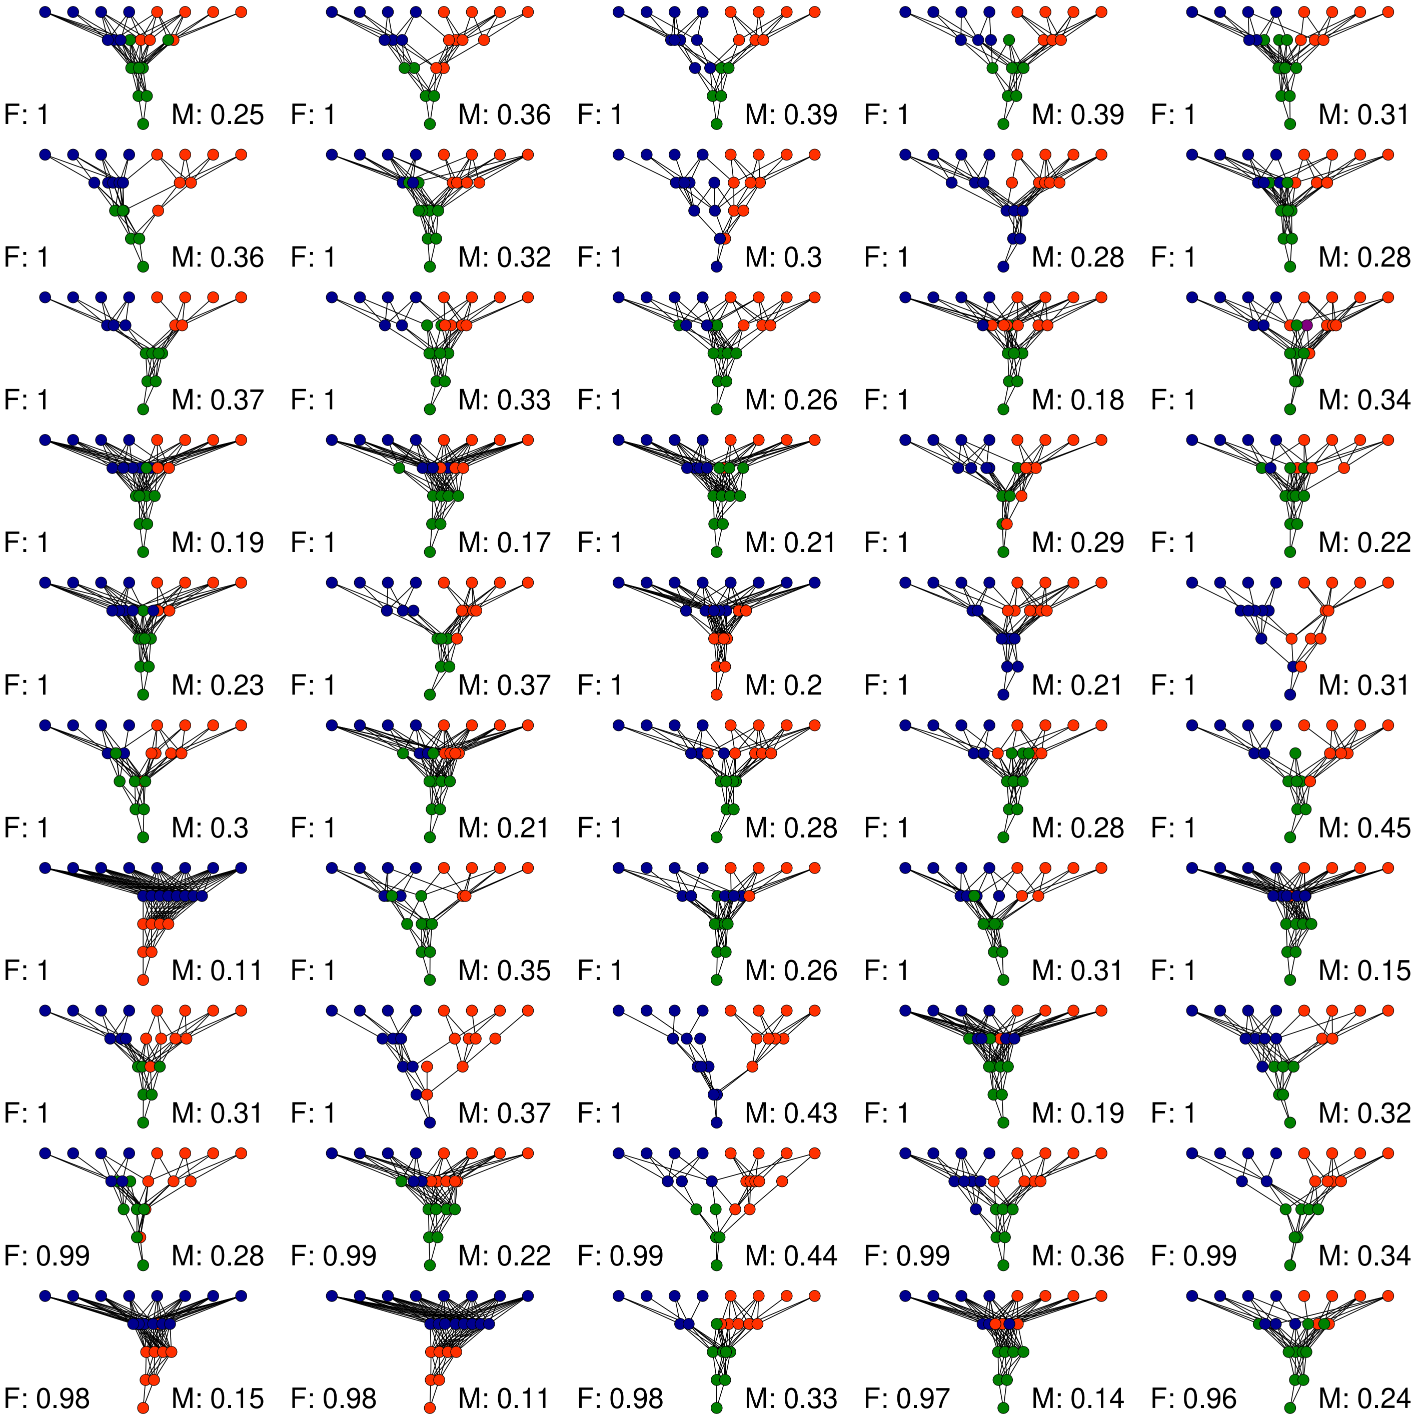


Figure 4: All 50 evolved neural networks from the retina experiment, with the *UserMod* treatment

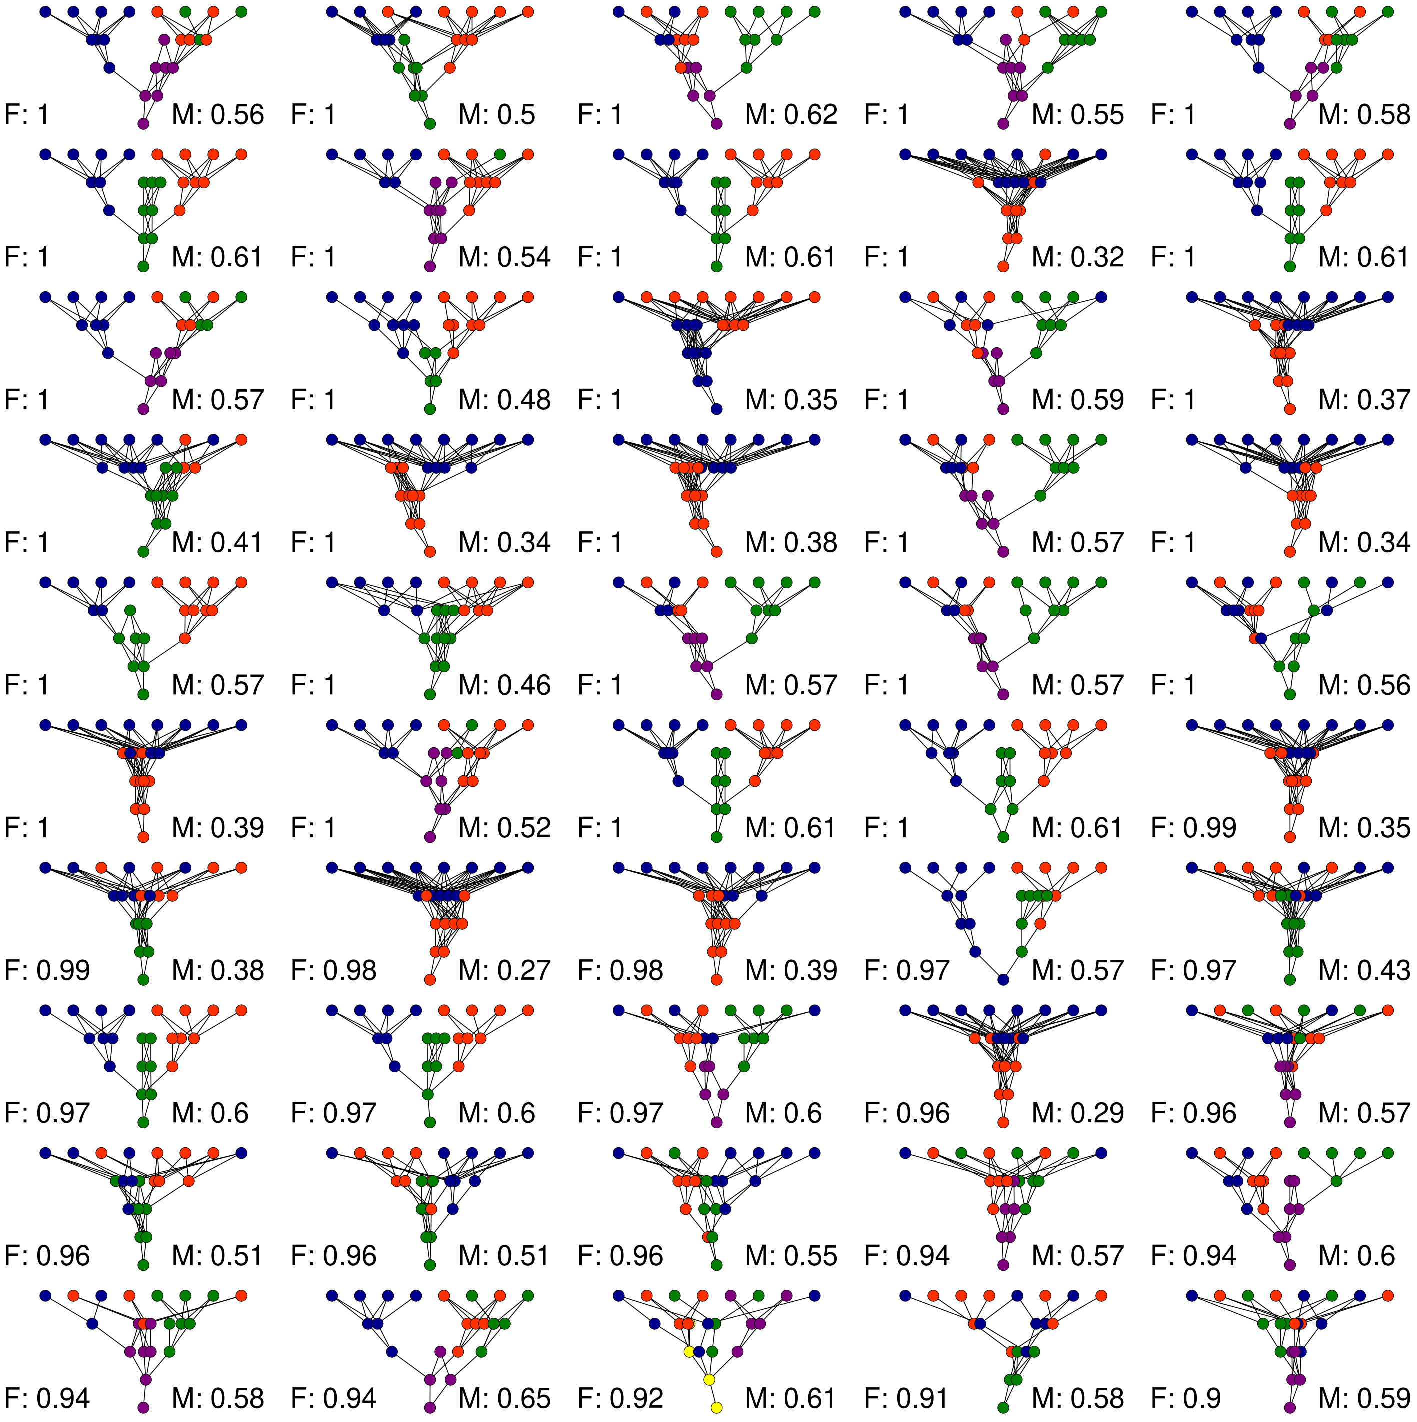


Figure 5: All 50 evolved neural networks from the retina experiment, with the *Q-Mod* treatment

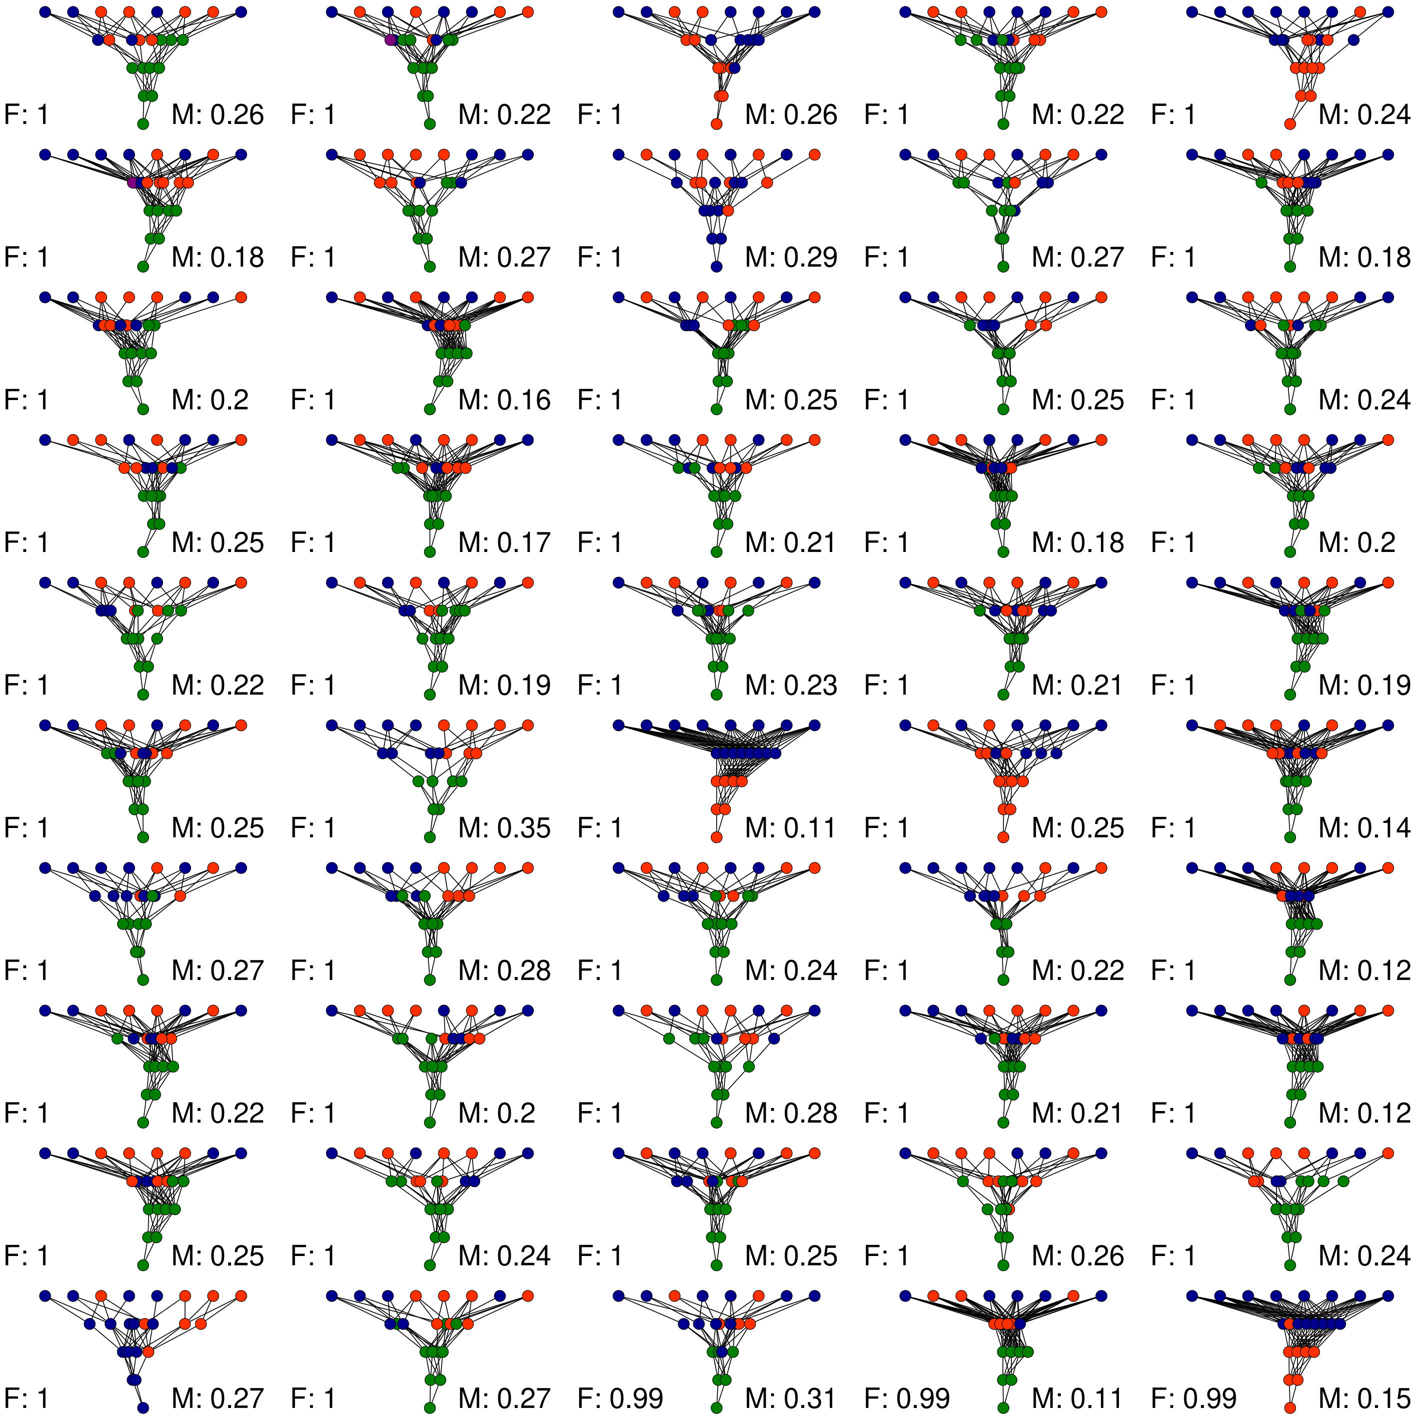


Figure 6: All 50 evolved neural networks from the retina experiment, with the *ModDiv* treatment

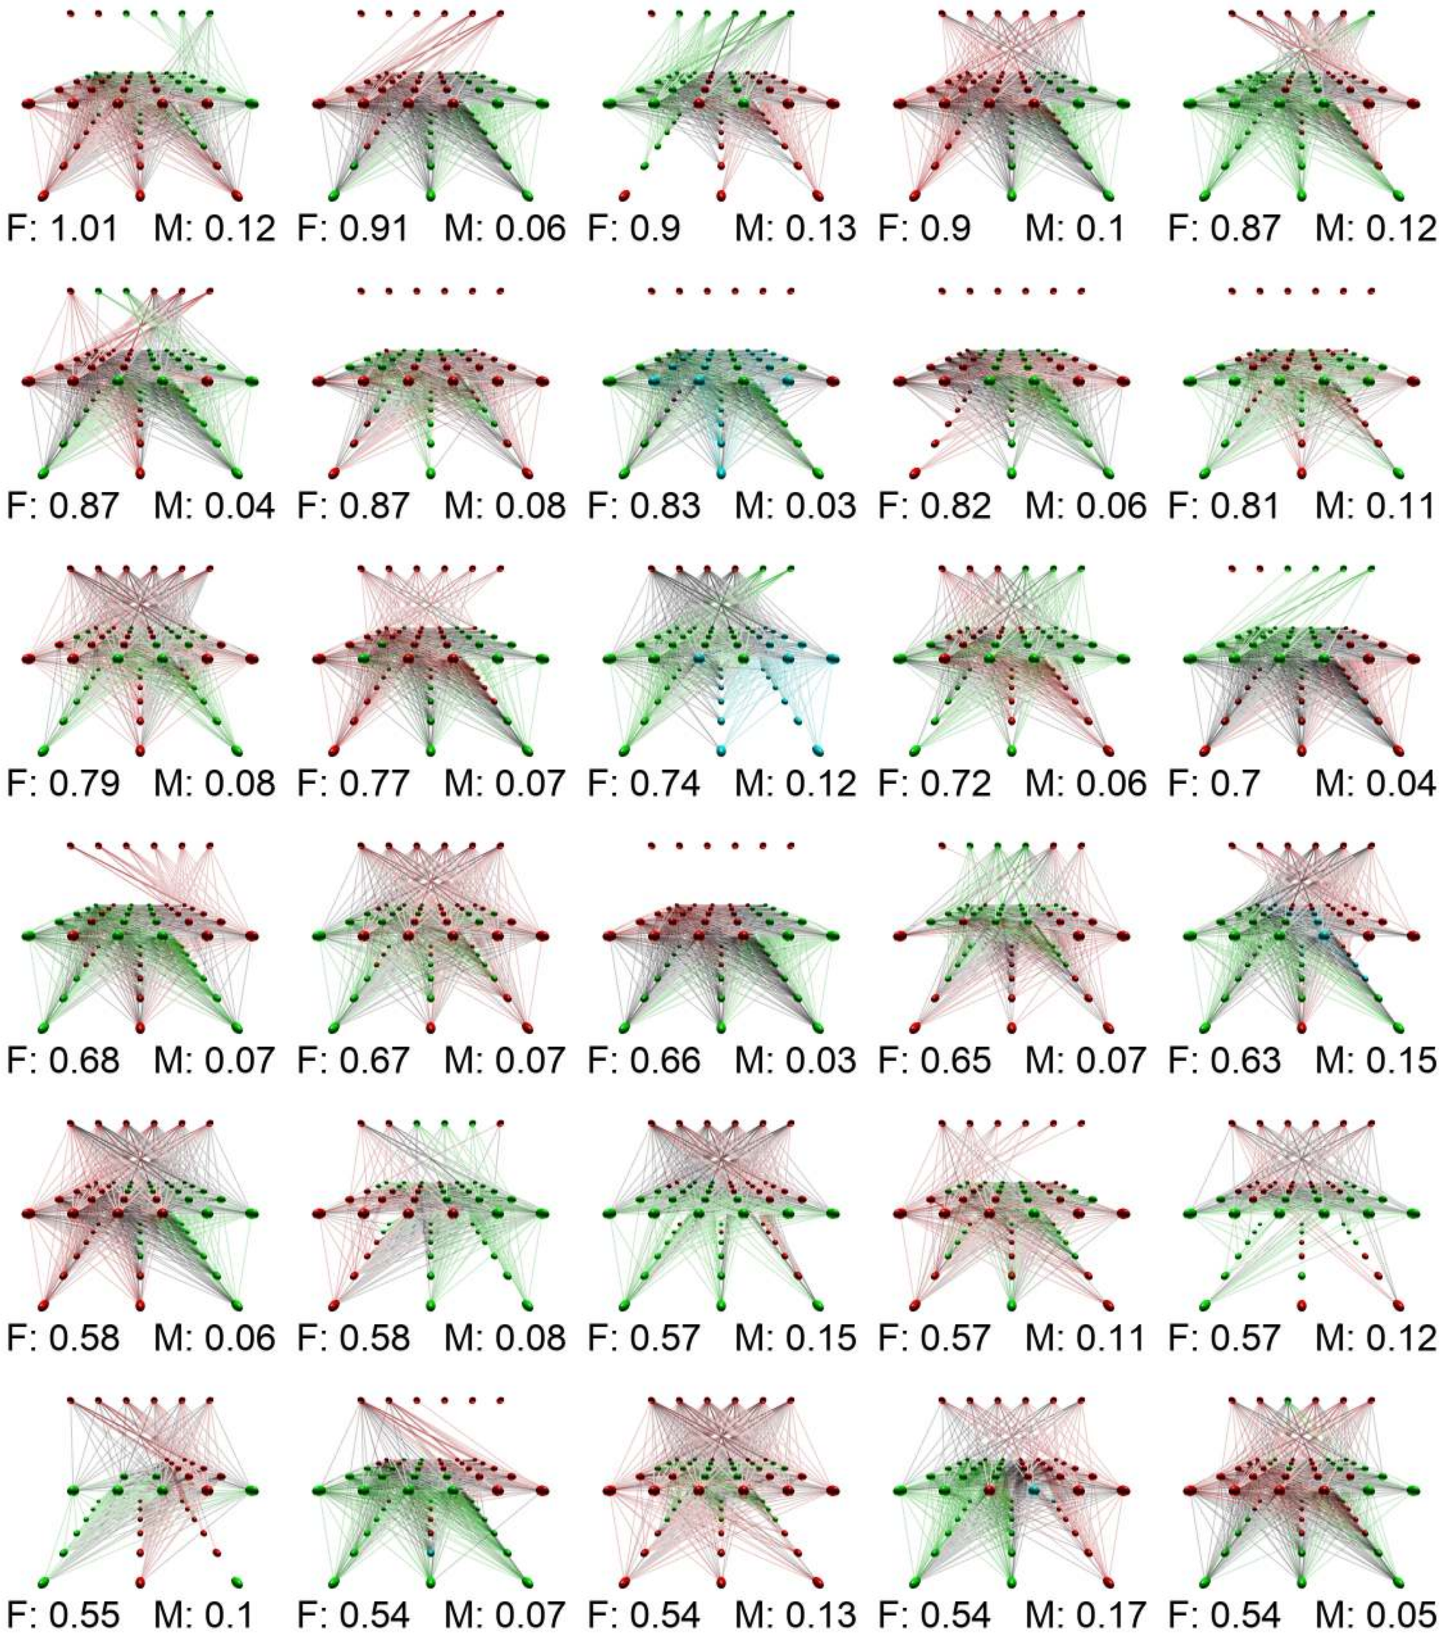


Figure 7: All 50 evolved neural networks from the robot locomotion experiment, with the *PA* treatment. (Part 1 of 2)

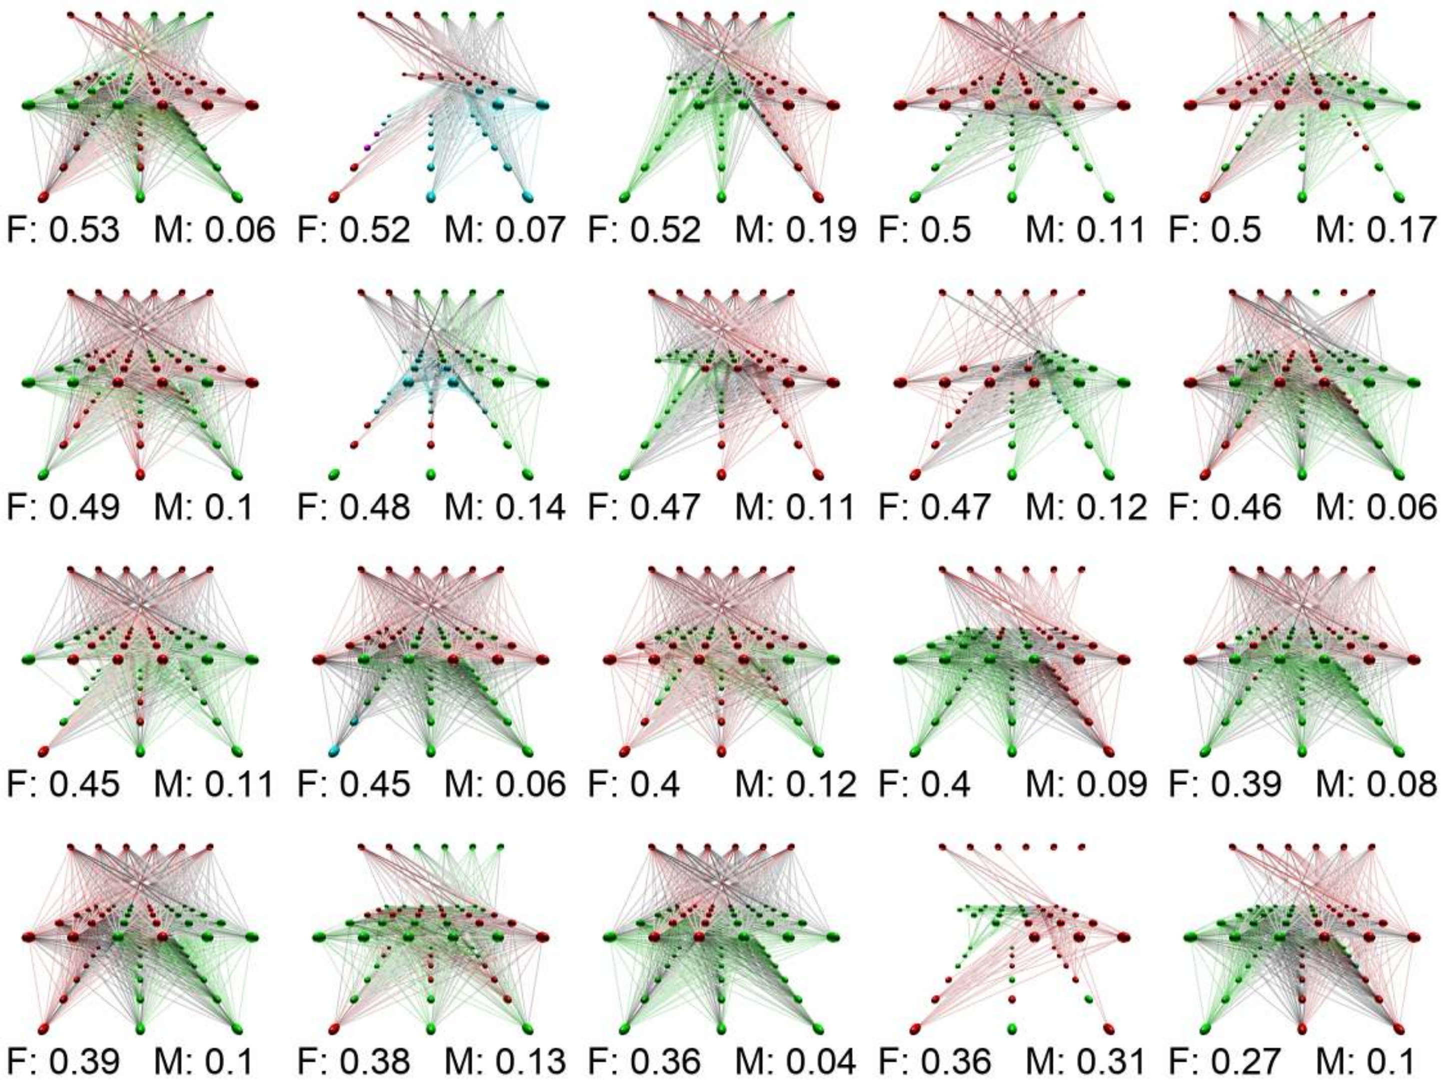


Figure 8: All 50 evolved neural networks from the robot locomotion experiment, with the *PA* treatment. (Part 2 of 2)

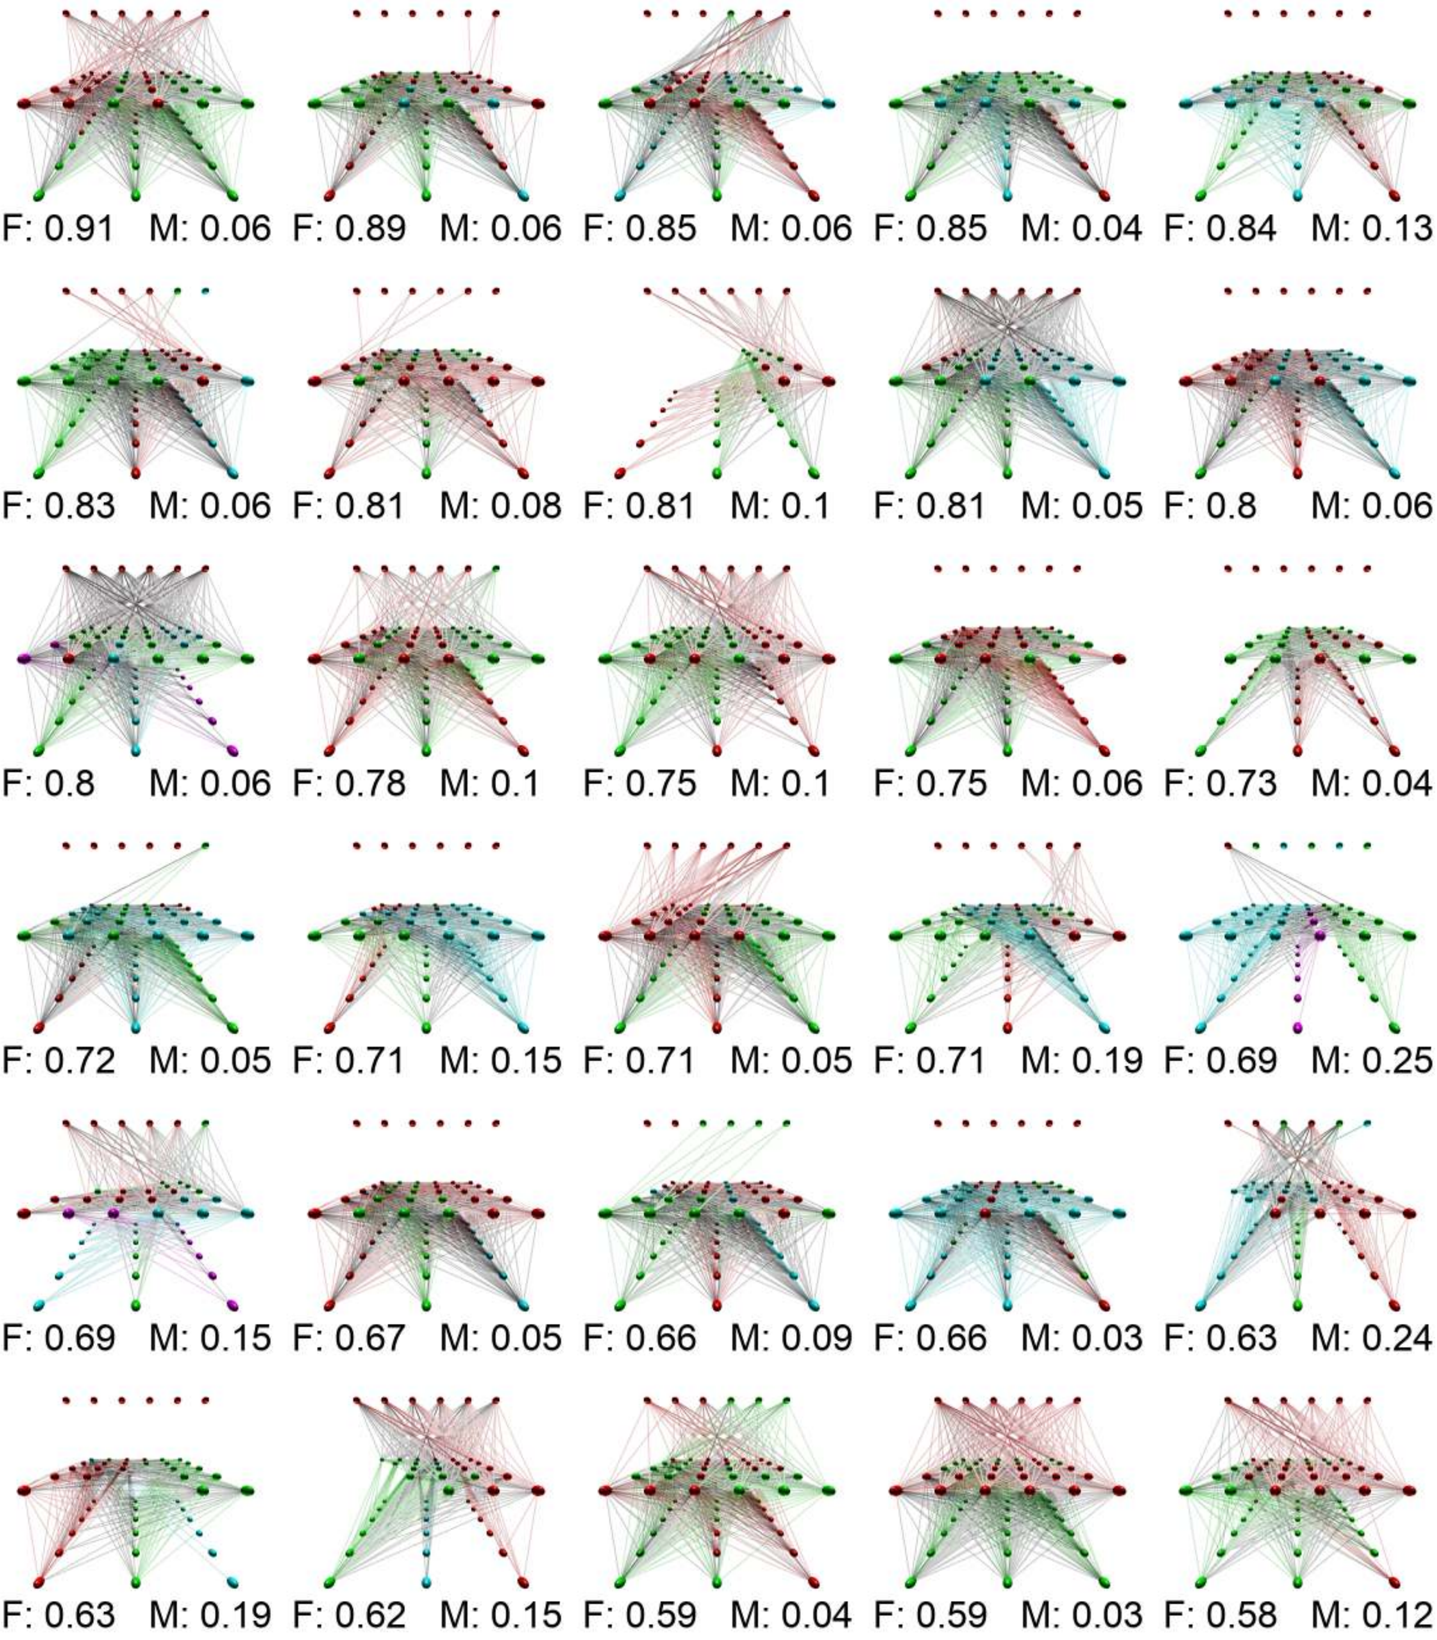


Figure 9: All 50 evolved neural networks from the robot locomotion experiment, with the *UserMod* treatment (Part 1 of 2)

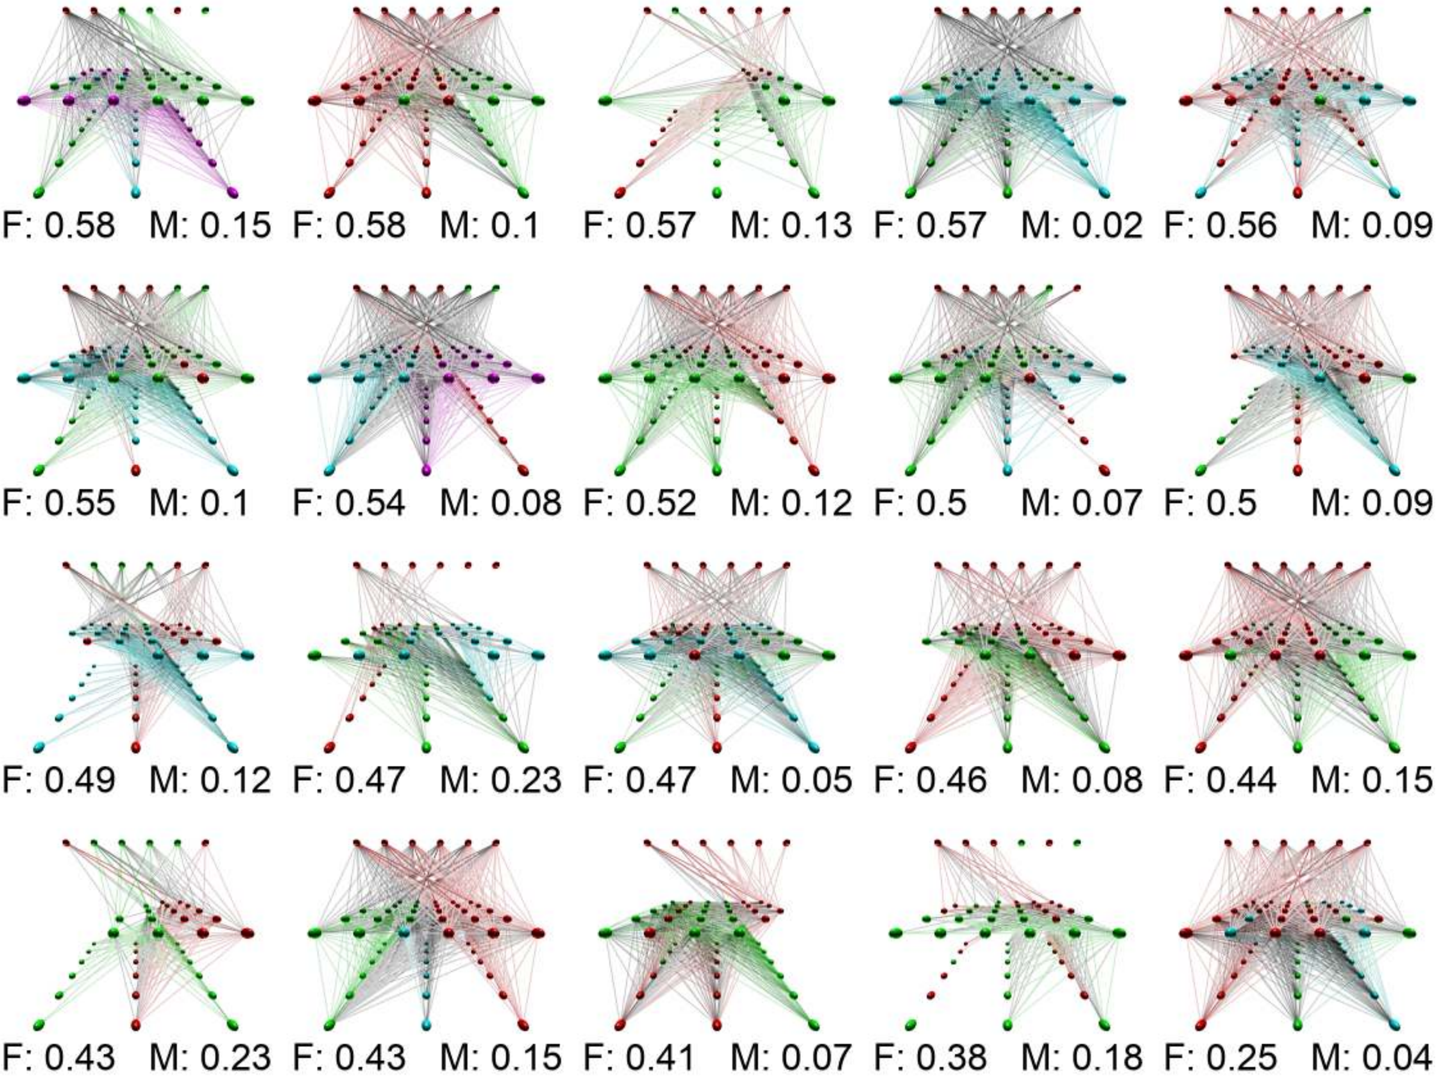


Figure 10: All 50 evolved neural networks from the robot locomotion experiment, with the *UserMod* treatment (Part 2 of 2)

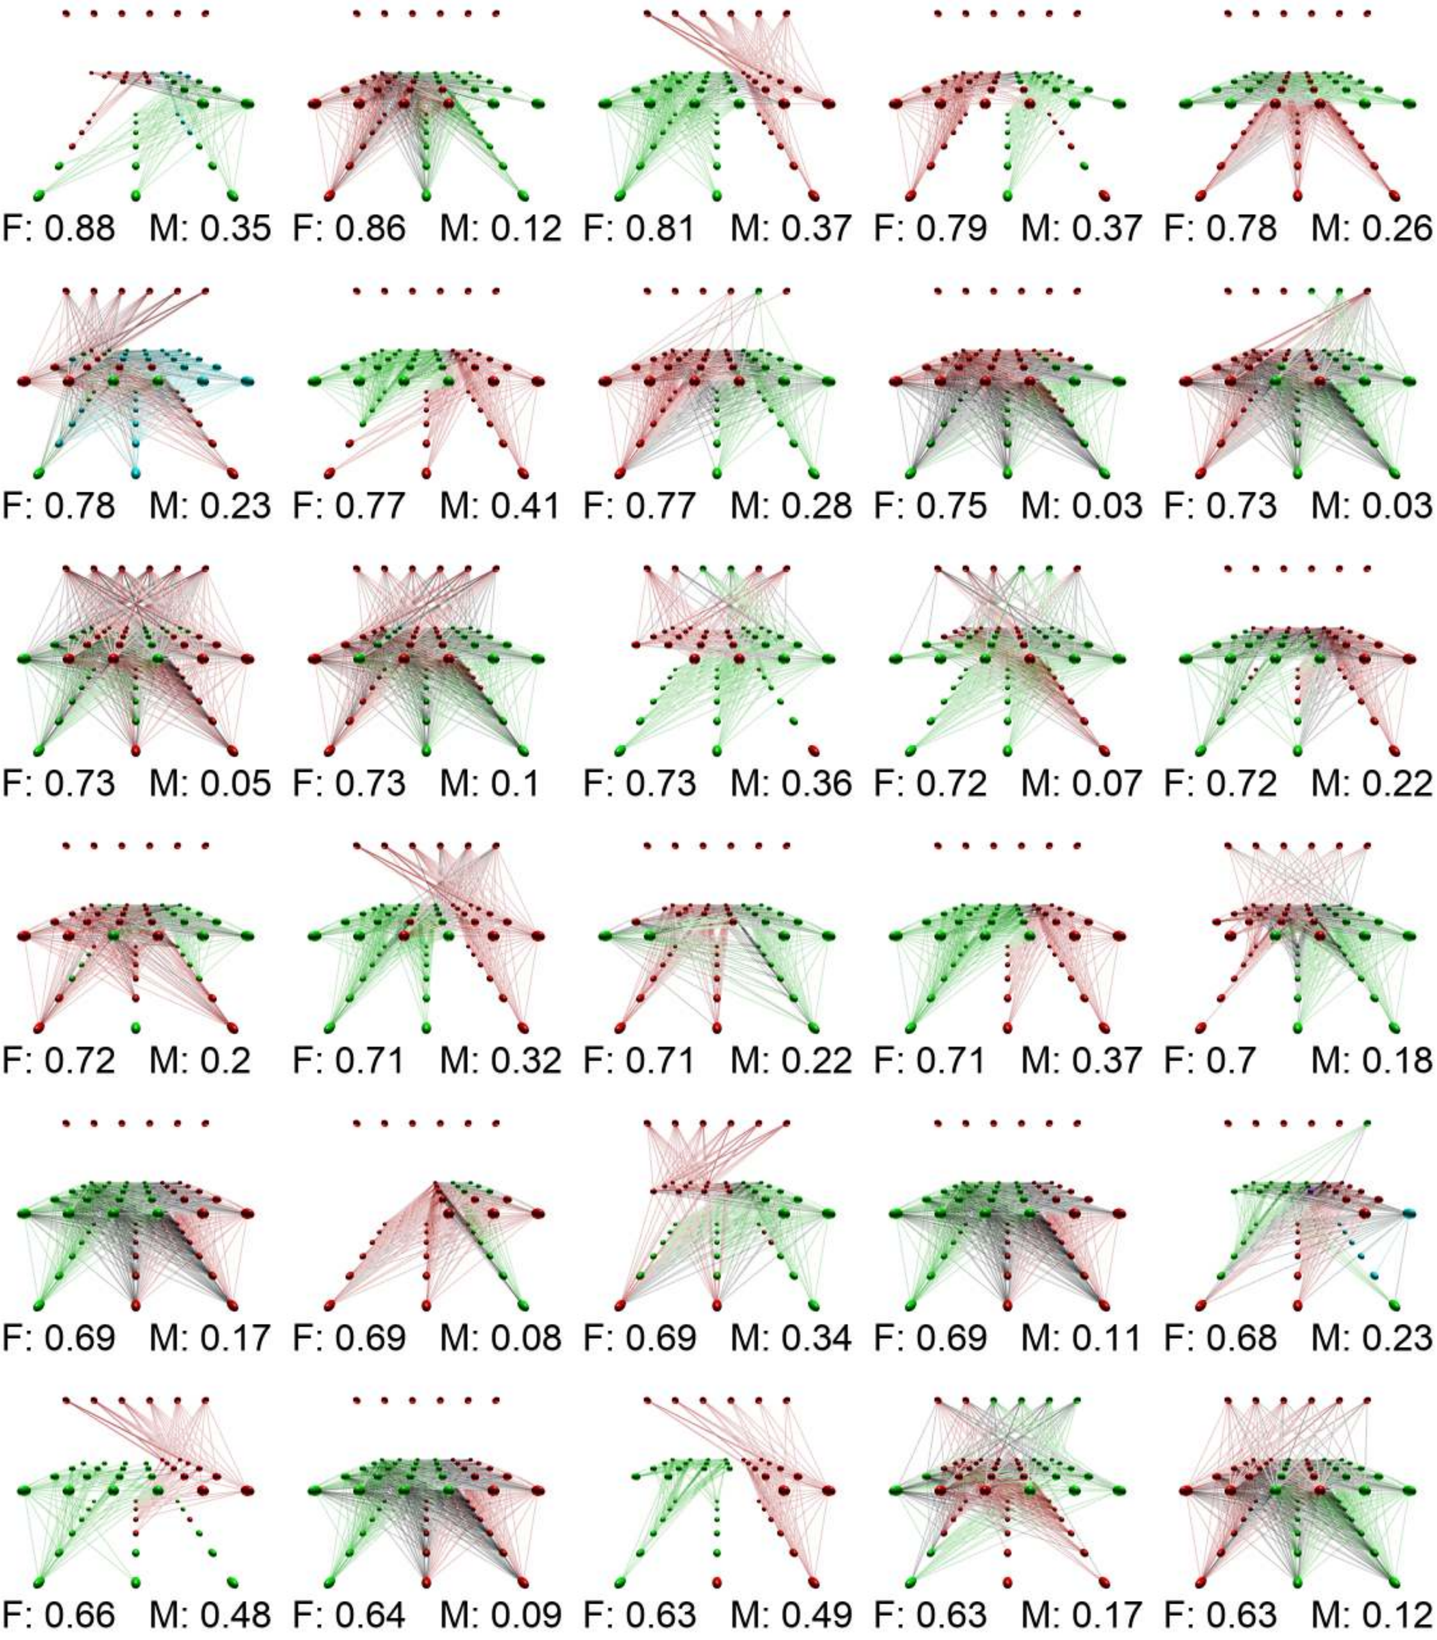


Figure 11: All 50 evolved neural networks from the robot locomotion experiment, with the *Q-Mod* treatment (Part 1 of 2).

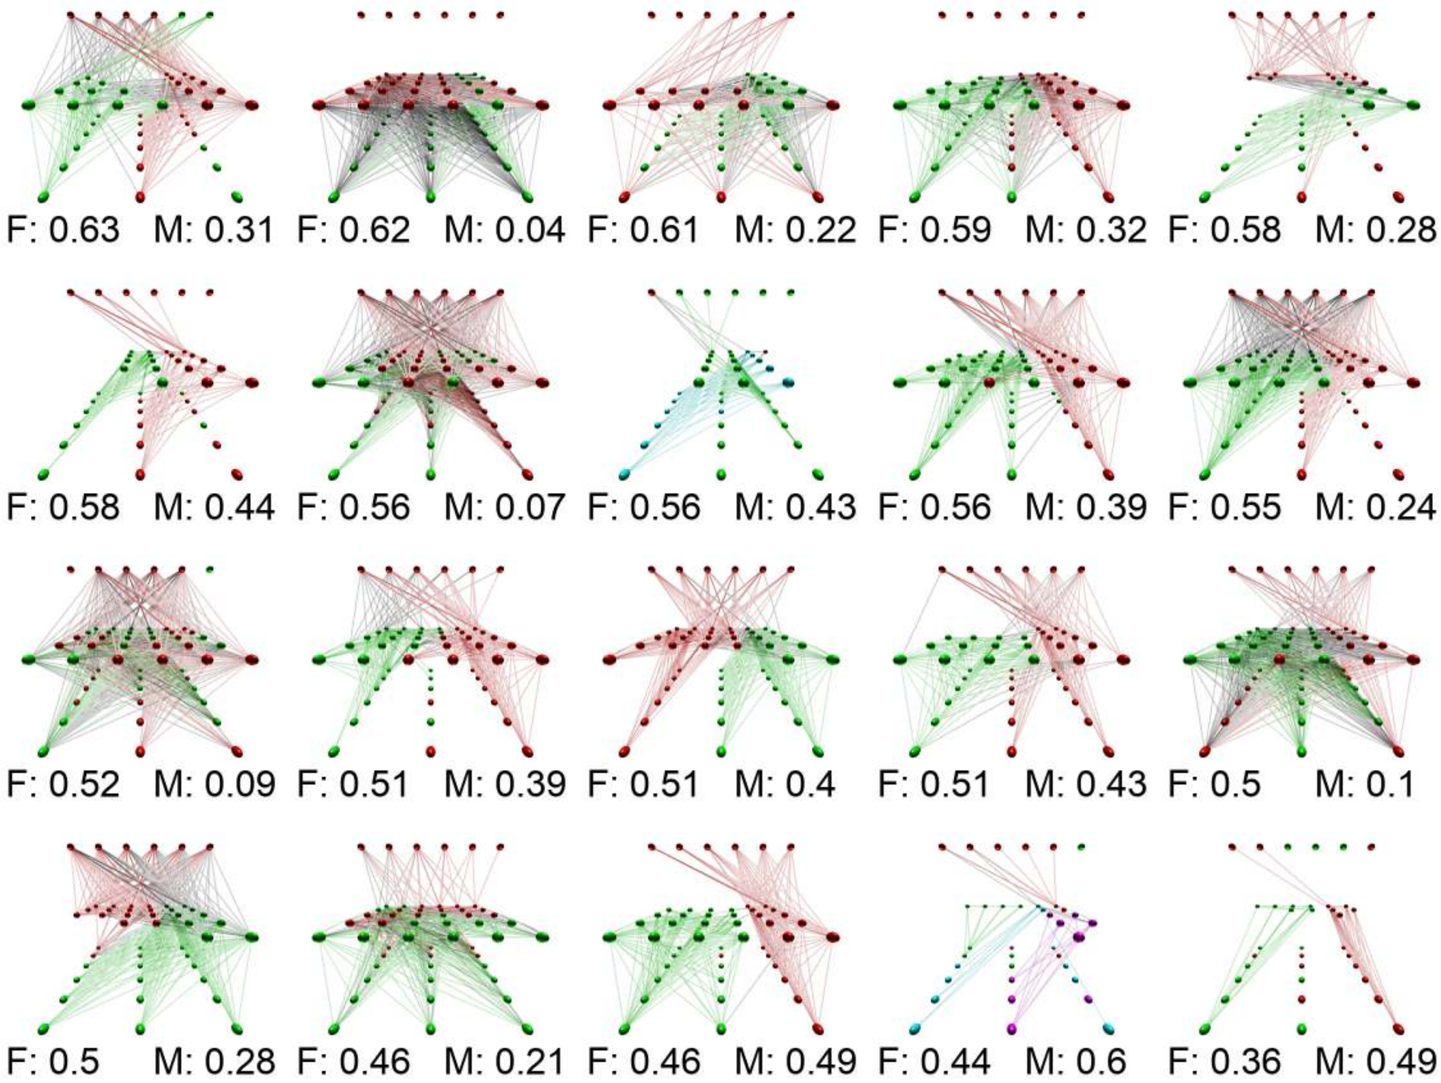


Figure 12: All 50 evolved neural networks from the robot locomotion experiment, with the *Q-Mod* treatment (Part 2 of 2).

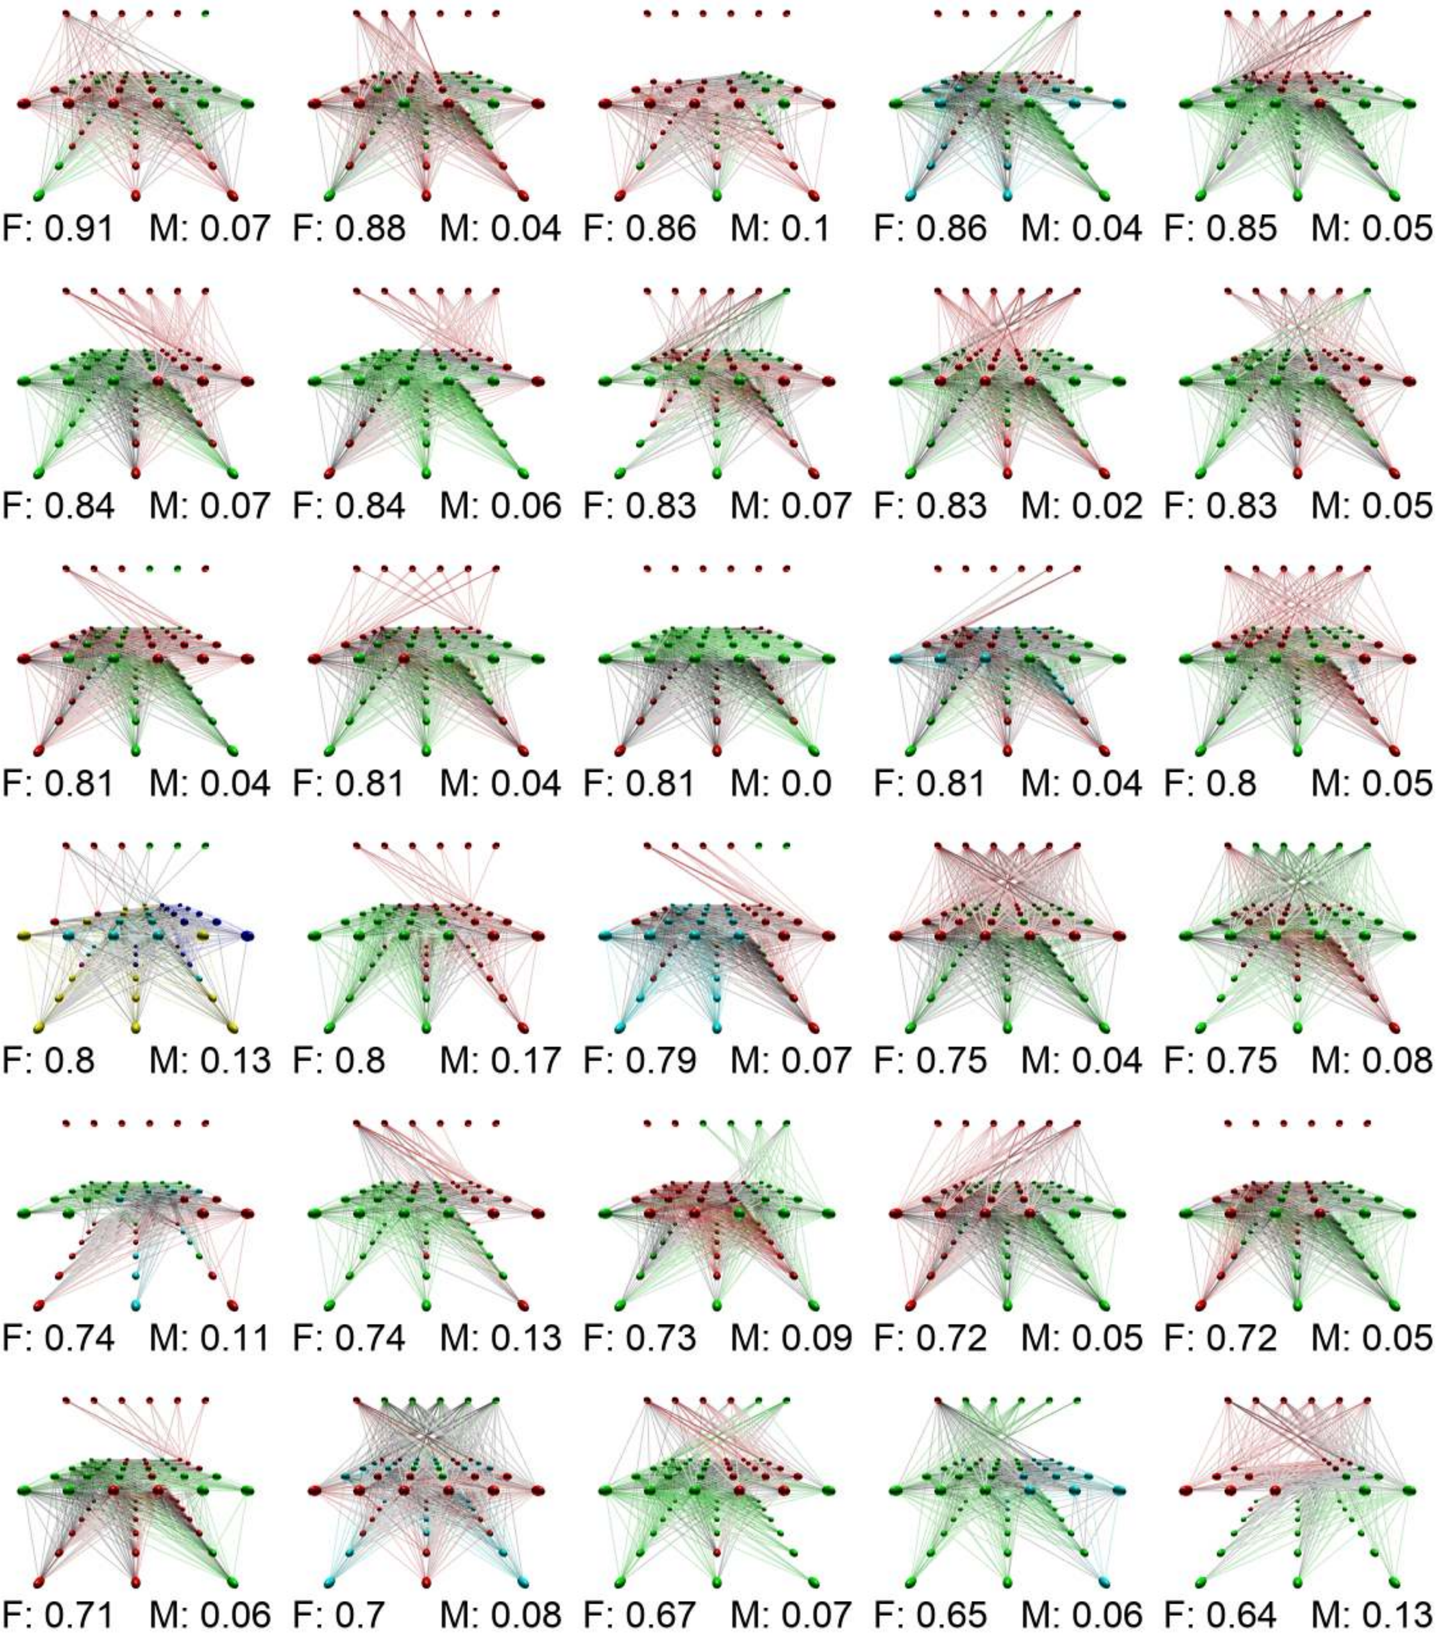


Figure 13: All 50 evolved neural networks from the robot locomotion experiment, with the *ModDiv* treatment (Part 1 of 2).

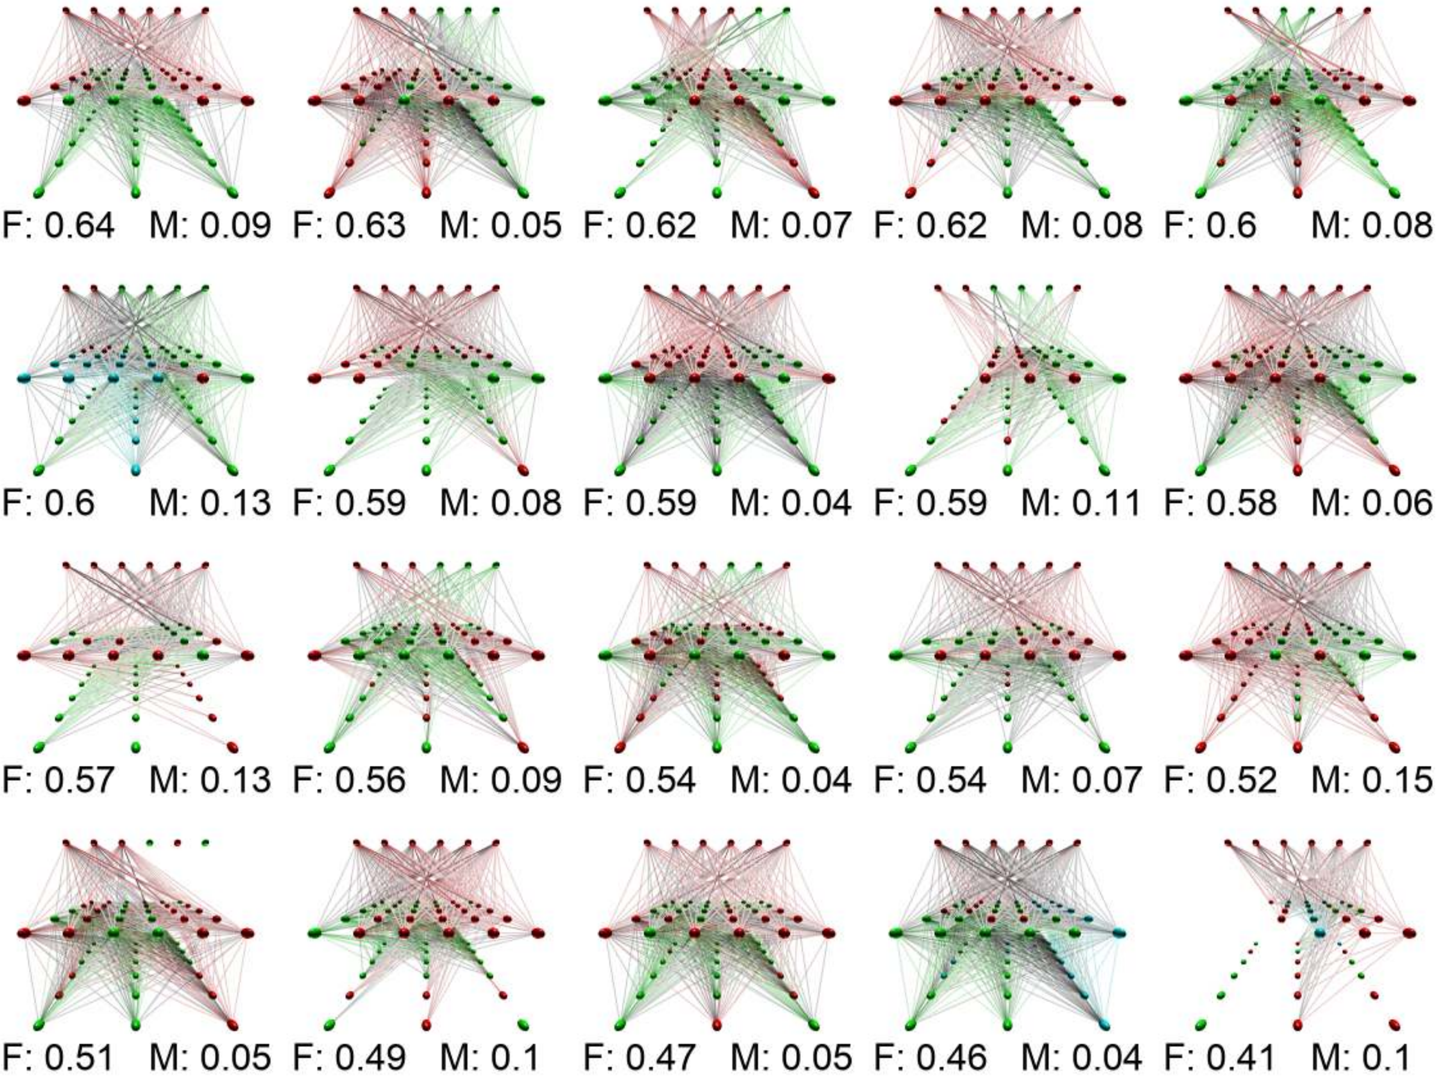


Figure 14: All 50 evolved neural networks from the robot locomotion experiment, with the *ModDiv* treatment (Part 2 of 2).

## References


Beer, R. D. and Gallagher, J. C. (1992). Evolving dynamical neural networks for adaptive behavior. *Adaptive behavior*, 1(1):91.

Clune, J., Mouret, J.-B., and Lipson, H. (2013). The evolutionary origins of modularity. *Proceedings of the Royal Society of London. Series B: Biological Sciences*, 280(1755):20122863.

Deb, K. (2001). *Multi-Objective Optimization Using Evolutionary Algorithms*, volume 6.

Huizinga, J., Mouret, J.-B., and Clune, J. (2016). Does Aligning Phenotypic and Genotypic Modularity Improve the Evolution of Neural Networks? In *Proceedings of the 2016 on Genetic and Evolutionary Computation Conference - GECCO '16*, pages 125–132.

Pugh, J. K. and Stanley, K. O. (2013). Evolving multimodal controllers with hyperneat. In *Proceedings of the 15th annual conference on Genetic and evolutionary computation*, pages 735–742. ACM.
